# Supplementary material for: Quantum Multiplexers, Parrondo Games, and Proper Quantization
Source: arXiv:0906.0645 source file (2009-06-03)
Supplement: Supplementary file 1 [file Appendix3.tex]

\chapter{An Alternative Quantization of the History Dependent Parrondo Game}

Following the authors of \cite{Flitney:02}, we restrict our attention to the details of the HD game with only 2 histories. The arbitrary case for $n-1$ histories can be got easily by generalization.

The classical game is embedded in the quantized game via identification of outcomes of the classical game with the basis states of the complex projective Hilbert space $\mathbb{H}^{\otimes 3}$ of qubits. We fix the basis of $\mathbb{H}^{\otimes 3}$ to be the ordered computational basis 
$$
\mathcal{B}=\left\{ \ket{000}, \ket{001}, \ket{010}, \ket{011}, \ket{100}, \ket{101}, \ket{110}, \ket{111} \right\}
$$
%\begin{figure}\centerline{
% \Qcircuit @C1em @R=.8em {
%&\ctrlo{+1} &\qw &\ctrlo{+1} &\qw &\ctrl{+1} &\qw &\ctrl{+1} &\qw \\
%  &\ctrlo{+1} &\qw &\ctrl{+1} &\qw &\ctrlo{+1} &\qw &\ctrl{+1} &\qw\\
%  &\gate{g_0} &\qw &\gate{g_1} &\qw &\gate{g_2} &\qw &\gate{g_3} &\qw \\}}
%\caption{\footnotesize{A quantum circuit representation of the block diagonal unitary operator used in the FNA protocol.}}
%\label{3rd ord mult}
%\end{figure}
We take $\ket{0}$ to represent a loss and $\ket{1}$ to represent a win. The first two qubits in an element of $\mathcal{B}$ represent the history of the game, while the last qubit represents the outcome of at the present stage of the game.
Consider the subset $\mathcal{W}=\left(\ket{001}, \ket{011}, \ket{101}, \ket{111}\right)$ of $\mathcal{B}$ in which the final qubit is always in the state $\ket{1}$. The elements of $\mathcal{W}$ represent a winning outcome in the classical game.

As in the FNA, the matrix for the quantized HD Parrondo game is
\begin{equation}\label{eqn:eq15}
X=\left( {{\begin{array}{*{20}c}
 {X_1 } \hfill & 0 \hfill & 0 \hfill & 0 \hfill \\
 0 \hfill & {X_2 } \hfill & 0 \hfill & 0 \hfill \\
 0 \hfill & 0 \hfill & {X_3} \hfill & 0 \hfill \\
 0 \hfill & 0 \hfill & 0 \hfill & {X_4 } \hfill \\
\end{array} }} \right)
\end{equation}
with 
\begin{equation}\label{eqn:eq16}
X_{j}=\left( {{\begin{array}{*{20}c}
a_j \hfil & b_j \hfill \\
-\overline{b}_j \hfill & \overline{a}_j \hfill \\
\end{array}} } \right)
\end{equation}

and $a_j, b_j \in \mathbb{C}$ satisfying $\left|a_j\right|^2+\left|b_j\right|^2=1$.

However, unlike FNA, we take the initial state of three qubits to be un-entangled, say 
\begin{equation}\label{unentangled state}
\left|q_1q_2q_3\right\rangle= \left( {{\begin{array}{c}
q_{11} \\
q_{12} \\
\end{array}} } \right) \otimes \left( {{\begin{array}{c}
q_{21} \\
q_{22} \\
\end{array}} } \right) \otimes \left( {{\begin{array}{c}
q_{31} \\
q_{32} \\
\end{array}} } \right);  \hspace{.2in} \left|q_{k1}\right|^2+\left|q_{k2}\right|^2=1; \hspace{.2in} k=1,2,3.
\end{equation}

We point out here that if the initial state of the qubits was the maximally entanglement state, then a single play of the quantum HD game will {\it not} preserve the classical game due to destruction of the histories of the game. The initial state may be written as a vector in $\mathbb{H}^{\otimes 3}$.
\begin{equation}\label{vector form}
\left|q_1q_2q_3\right\rangle= \left( {{\begin{array}{c}
q_{11}q_{21}q_{31}\\
q_{11}q_{21}q_{32}\\
q_{11}q_{22}q_{31}\\
q_{11}q_{22}q_{32}\\
q_{12}q_{21}q_{31}\\
q_{12}q_{21}q_{32}\\
q_{12}q_{22}q_{31}\\ 
q_{12}q_{22}q_{32}
\end{array}} } \right); \hspace{.2in}  \sum_{r,s,t=1}^2\left|q_{1r}q_{2s}q_{3t}\right|^2=1
\end{equation}

The output from the quantum HD Parrondo game for the input state in expression (\ref{vector form}) is 

\begin{equation}\label{output}
\left|q_1q_2q_3\right\rangle= \left( {{\begin{array}{c}
q_{11}q_{21}\left(a_1q_{31}+b_1q_{32}\right)\\
q_{11}q_{21}\left(\overline{a}_1q_{32}-\overline{b}_1q_{31}\right)\\
q_{11}q_{22}\left(a_2q_{31}+b_2q_{32}\right)\\
q_{11}q_{22}\left(\overline{a}_2q_{32}-\overline{b}_2q_{31}\right)\\
q_{12}q_{21}\left(a_3q_{31}+b_3q_{32}\right)\\
q_{12}q_{21}\left(\overline{a}_3q_{32}-\overline{b}_3q_{31}\right)\\
q_{12}q_{22}\left(a_4q_{31}+b_4q_{32}\right)\\ 
q_{12}q_{22}\left(\overline{a}_4q_{32}-\overline{b}_4q_{31}\right)
\end{array}} } \right) 
\end{equation}

with the normalizing condition taking the form
\begin{eqnarray*}
&\left|q_{11}\right|^2\left(\sum_{s=1}^2\left|q_{2s}\left(a_sq_{31}+b_sq_{32}\right)\right|^2+\left|q_{2s}\left(\overline{a}_sq_{32}-\overline{b}_sq_{31}\right)\right|^2\right) \\  &+\left|q_{12}\right|^2\left(\sum_{s=1}^2\left|q_{2s}\left(a_{s+2}q_{31}+b_{s+2}q_{32}\right)\right|^2+\left|q_{2s}\left(\overline{a}_{s+2}q_{32}-\overline{b}_{s+2}q_{31}\right)\right|^2\right)=1
\end{eqnarray*} 

Note that the output or final state in (\ref{output}) exhibits entanglement between the qubits. The probability of winning, $p_{\rm{win}}^Q$ is the sum of the amplitudes of the coefficients of the elements of $\mathcal{W}$ in (\ref{output}), namely,
\begin{equation}\label{p of win}
p_{\rm{win}}^{Q}=\left|q_{11}\right|^2\left(\sum_{s=1}^2\left|q_{2s}\right|^2\left|\overline{a}_sq_{32}-\overline{b}_sq_{31}\right|^2\right)+\left|q_{12}\right|^2\left(\sum_{s=1}^2\left|q_{2s}\right|^2\left|\overline{a}_{s+2}q_{32}-\overline{b}_{s+2}q_{31}\right|^2\right)
\end{equation}  

Switching to polar form of the complex numbers and using the conditions $\left|q_{k1}\right|^2+\left|q_{k2}\right|^2=\left|a_j\right|^2+\left|b_j\right|^2=1$ for all values of $j$ and $k$, we set
\begin{equation}\label{polar qk1}
q_{k1}=e^{i\phi_{q_{k}}}\cos\left(\frac{\theta_{q_{k}}}{2}\right)
\end{equation}
\begin{equation}\label{polar qk2}
q_{k2}=e^{i\eta_{q_{k}}}\sin\left(\frac{\theta_{q_{k}}}{2}\right)
\end{equation}

\begin{equation}\label{aj}
a_j= e^{i\phi_{j}}\cos\left(\frac{\theta_{j}}{2}\right)
\end{equation}
\begin{equation}\label{bj}
b_j=e^{i\eta_{j}}\sin\left(\frac{\theta_{j}}{2}\right)
\end{equation}

with $\theta_{q_{k}},\theta_j \in \left[0,\pi\right]$, $\eta_{q_{k}},\eta_j, \phi_{q_{k}}, \phi_j \in \left[0,2\pi\right]$.  

These substitutions allow us to reduce 
\begin{equation}\label{mid term}
\left|\overline{a}_jq_{32}-\overline{b}_jq_{31}\right|^2 =  \cos^2\left(\frac{\theta_j}{2}\right)\sin^2\theta_{q_{3}}+\sin^2\left(\frac{\theta_j}{2}\right)\cos^2\theta_{q_{3}}-2\Re\left\{a_j\overline{b}_jq_{31}\overline{q}_{32}\right\}
\end{equation}

with
$$
\Re\left\{a_j\overline{b}_jq_{31}\overline{q}_{32}\right\}=\cos\left(\theta_j-\eta_j+\phi_{q_{3}}-\eta_{q_{3}}\right)\cos\left(\frac{\theta_j}{2}\right)\sin\left(\frac{\theta_j}{2}\right)\cos\theta_{q_{3}}\sin\theta_{q_{3}}
$$
Substituting equations (\ref{polar qk1}) - (\ref{mid term}) into equation (\ref{p of win}) allows us to express $p_{\rm{win}}^Q$ in terms of {\it twenty one} real variables, each taking on values from the closed unit interval, versus only four such variable that express $p_{\rm{win}}$. 

The expected payoff to the player in a single play of the classical HD Parrondo game is $2p_{\rm{win}}-1$ while in the quantum game it is $2p_{\rm{win}}^Q-1$. Quantization will enhance the payoff if $p_{\rm{win}}^Q > p_{\rm{win}}$. However, it is possible that for some range of values of some of the domain variables $p_{\rm{win}}^Q \leq p_{\rm{win}}$. In other words, the choice of initial state and the choice of the values of the phase variables in the unitary operator for the quantization lends the expected payoff a different behavior than the expected payoff in the classical game. 

\subsection{Equal Superposition as the Initial State}

Consider the following case in which the initial state is the equal superposition
\begin{equation}\label{equal super}
\left( {{\begin{array}{c}
\frac{1}{\sqrt{2}} \\
\frac{1}{\sqrt{2}} \\
\end{array}} } \right) \otimes 
\left( {{\begin{array}{c}
\frac{1}{\sqrt{2}} \\
\frac{1}{\sqrt{2}} \\
\end{array}} } \right) \otimes 
\left( {{\begin{array}{c}
\frac{1}{\sqrt{2}} \\
\frac{1}{\sqrt{2}}\\
\end{array}} } \right)=\frac{1}{\sqrt{8}}\left(1,1,1,1,1,1,1\right)^{T}.
\end{equation}
Then $p_{\rm{win}}^Q$ is simply

\begin{equation}\label{eqn19}
p_{\rm{win}}^{Q}=\frac{1}{8}\left(4-\sum_{j=1}^{4}\sin\theta_{j}\cos(\eta_j-\phi_j)\right)=\frac{1}{2}-\frac{1}{8}\sum_{j=1}^{4}\sin\theta_{j}\cos(\eta_j-\phi_j)
\end{equation}

For values of the phase angles $\eta_j, \phi_j$ such that $\sum_{j=1}^{4}\sin\theta_{j}\cos(\eta_j-\phi_j) >0$, the quantum game is losing. For values that satisfy $\sum_{j=1}^{4}\sin\theta_{j}\cos(\eta_j-\phi_j)<0$, the quantum game is winning, where as the game is fair when $\sum_{j=1}^{4}\sin\theta_{j}\cos(\eta_j-\phi_j) =0$.

The simplest case to analyze is when $\eta_j=\phi_j$ since in this case 
$$
p_{\rm{win}}^{Q}=\frac{1}{2}-\frac{1}{8}\sum_{j=1}^{4}\sin\theta_{j}
$$
and is equal to $\frac{1}{2}$ for $\theta_j=0$ or $\theta_j=\pi$, meaning that the quantum game is fair. However, $p_{\rm{win}}^{Q}$ is equal to $\frac{1}{2}-\epsilon$, $\epsilon > 0$, for all other values of the $\theta_j$, meaning that the game is losing.
