# Supplementary material for: Quantum Multiplexers, Parrondo Games, and Proper Quantization
Source: arXiv:0906.0645 source file (2009-06-03)
Supplement: Supplementary file 2 [file Appendix5.tex]

\chapter{Meyer's Quantum Penny Flip Game}

Two players engage in a simple penny flipping game, where the penny involved in fact a ``quantum penny,'' which is nothing more than a qubit. The stage on which Meyer's game is played is the starship Enterprise from the popular science fiction TV series {\it Star Trek: The Next Generation}, and the players are Captain Picard ($P$) and ``Q'' ($Q$), the two protagonists of the show. The player $Q$ is in fact an omnipotent entity, one of whose abilities is the ability to manipulate quantum mechanics. 

The game is played according to the following rules: the entity $Q$ asks $P$ to place the penny in a box, head up. Then beginning with $Q$, players $Q$ and $P$, respectively, take turns flipping the penny over, or not, with $Q$ making the third and final move. Player $Q$ wins if the penny is head up when the box is opened, $P$ otherwise. 

For a standard ``classical'' penny, this game can be expressed by the payoff Table \ref{class PQ} where rows and columns are $P$'s and $Q$'s pure strategies respectively.

\begin{table}
\begin{center}
  \begin{tabular}{|r|r|r|r|r|}
	  	 \hline
	    &$NN$ & $NF$ & $FN$ & $FF$\\
		  \hline
      $N$ & $-1$ & $1$ & $1$ & $-1$\\
      \hline
			$F$ & $1$ & $-1$ & $-1$ & $1$\\
			\hline
	  \end{tabular}
 \caption{\small{Classical $P$ and $Q$ penny flip game.}}
 \label{class PQ}
 \end{center}
\end{table}

For a game played with a qubit, let $\left\{H,T\right\}$ be identified with the orthonormal basis $\left\{\left|0 \right\rangle, \left|1\right\rangle \right\}$ of the state space of a qubit. The classical pure strategies of flip ($F$) and no-flip ($N$) of the players are now represented by the following matrices.
\begin{equation}
N: \quad \left(\begin{array}{cc}
1 & 0 \\
0 & 1
\end{array}\right), \quad
F: \quad \left(\begin{array}{cc}
0 & 1 \\
1 & 0
\end{array}\right)
 \label{classicalStrategies}%
\end{equation}
A mixed strategy is described by the matrix
\begin{equation}
\quad \left(\begin{array}{cc}
1-p & p \\
p & 1-p
\end{array}\right)
 \label{MixedStrategy}%
\end{equation}
where $p\in\left[  0,1\right]  $ is the probability with which the player
flips the coin. A sequence of mixed strategies puts the state of the coin into a
convex linear combination $q\left|0\right\rangle+(1-q)\left|1\right\rangle$ where $0\leq q\leq1$. %The coin is then
%in state $\left|0\right\rangle$ with probability $q$ and in state $(1-q)$ with probability $(1-p)$. Player $Q$ plays his move first, after $P$ puts
%the coin in the state $H$.

Player $Q$ decides to exercise his omnipotence and manipulate the quantum penny quantum mechanically by a sequence of unitary rather
than stochastic matrices. In general, a qubit is in a superposition of the basis state of the coin: $a\left|  0\right\rangle +b\left|  1\right\rangle $ where $a,b\in\mathbb{C}$ and $a\bar a+b \bar b=1$. Given the penny is initially in the state $\left|  0\right\rangle $, the
following special unitary action $U$ by $Q$ puts the penny into the state
$a\left|  0\right\rangle +b\left|  1\right\rangle $:%
\begin{equation}
\left(\begin{array}{cc}
a & b \\
- \bar b & \bar a \end{array}\right).
\label{Q's action}
\end{equation}

Using density matrix notation, the initial state of the coin can be
written as
\begin{equation}
\rho_{0}=\left|  0\right\rangle \left\langle 0\right|
\end{equation}
Player $Q$'s special unitary action $U$ changes the state $\rho_{0}$ to%
\begin{equation}
\rho_{1}=U\rho_{0}U^{\dag}=\left(
\begin{array}
[c]{cc}%
a \bar a & a \bar b\\
b \bar a & b \bar b
\end{array}
\right)
\end{equation}
because unitary transformations act on density matrices by conjugation. Player $P$
is restricted to use only a classical mixed strategy (\ref{MixedStrategy}) by
flipping the coin with probability $p$. After his action the coin is in the
pure state $b\left|  0\right\rangle +a\left| 1\right\rangle$ with
probability $p$ and in the pure state $a\left|  0\right\rangle +b\left|
1\right\rangle$ with probability $(1-p)$. Player $P$'s mixed action acts on this density matrix, not as a stochastic
matrix on a probabilistic state, but as a convex linear combination of
unitary (deterministic) transformations:
\begin{align}
\rho_{2}  &  =pF\rho_{1}F^{\dagger}+(1-p)N\rho_{1}N^{\dagger}\nonumber\\
&  =\left(
\begin{array}
[c]{cc}%
pb{\bar b}+(1-p)a{\bar a} & pb{\bar a}+(1-p)a{\bar b}\\
pa{\bar b}+(1-p)b{\bar a} & pa{\bar a}+(1-p)b{\bar b}%
\end{array}
\right)
\end{align}
Now $Q$ has at his disposal the following move:
\begin{equation}
U_{1}=\frac{1}{\sqrt{2}}\left(
\begin{array}
[c]{cc}%
1 & 1\\
1 & -1
\end{array}
\right)
\end{equation}
that puts the coin into a simultaneous eigenstate (with eigenvalue $1$) of both $F$ and $N,$ which then becomes an invariant under any mixed strategy
of $P$. In his second action $Q$ acts again with $U$, which is its own inverse, and gets back the state 
$\rho_{0}=\ket{0}$ and wins.
